# Supplementary material for: Face, Body, Voice: Video Person-Clustering with Multiple Modalities
Source: arXiv:2105.09939 source file (2021-05-20)
Supplement: Supplementary file 1 [file Supplementary_Video_Contents.tex]

Three videos are included with this supplementary material. Here, we explain what is contained in each of them. 

The first is titled, ``Story\_Understanding''. This video highlights the advantages of the new task of multi-modal video person-clustering, over the established, more limited task of face-clustering. The video visualises the amount of information that is used by these two tasks. For the face-clustering task, only information from visible faces is used. This omits important information such as characters viewed from behind, or from the audio track. This limits the utility of the resulting clusters for downstream applications such as story understanding. The multi-modal person-clustering task on the other hand uses all available cues (\ie face, body and voice). Clearly, a person-level understanding is essential for downstream applications of grouping-by-identity such as story understanding.

The second is titled ``VPCD\_Contents''. This video visualises the different annotations provided in \dnameemphasis, namely the face-tracks, body-tracks (from front and behind), and voice-tracks. The video shows clips containing example annotations from all 6 program sets in \dnameemphasis. Every face-body pair belonging to the same person-track is drawn with the same color. Note,  \dnameemphasis covers a diverse set of characters in a variety of scenes (\eg including dark scenes in Sherlock, Hidden Figures), various viewpoints and over-the-shoulder shots. 

The third video, titled ``MuHPC\_Results'' shows a selection of \mnameMM person-clustering results from \dnameemphasis. In each clip, tracks are marked with a unique cluster ID number and colour, which signify which cluster they belong to. Particularly of note are the multiple backs of people that are clustered correctly \ie Ross (cluster 2) in the first clip from Friends, Penny (cluster 3) in the second clip from TBBT, and the multiple backs in the dark scene from Buffy. Impressively, the very small Chandler, Joey and Ross tracks (clusters 1,0,2, respectively) at the back of the shot at the end of the Friends clip, are correctly clustered with other tracks of the same character.
