# Supplementary material for: Face, Body, Voice: Video Person-Clustering with Multiple Modalities
Source: arXiv:2105.09939 source file (2021-05-20)
Supplement: Supplementary file 2 [file supplementary.tex]

In this work, we propose \datasetname (\dname), a composite dataset for multi-modal person-clustering in videos. 
This is described in Section 4 in the main manuscript. Here, we provide more details.

%%%%%%%%%%%%%%%%%%%%%%%%%%%%%%%%%%%%%%%
\subsection{Data Collection and Features}
\label{sub:data_collection}
%%%%%%%%%%%%%%%%%%%%%%%%%%%%%%%%%%%%%%%
In this section, we describe in more details the process for acquiring annotated body tracks and speech-turns for the datasets in \dname, as well as the features extracted.

\paragraph{Face-Tracks \& Features.}
In all cases, we use the same annotated face-tracks that were provided by the comprising dataset. 
In line with~\cite{Kalogeiton20,ball} we extract 256D face identity discriminating features from the face detections in each face-track using an SENet50 architecture~\cite{hu2018squeeze} (pre-trained on MS-Celeb-1M~\cite{guo2016ms} and fine-tuned on VGGFace2~\cite{Cao18}). 
In the cases of TBBT, Buffy, Friends, and Sherlock (1-4) we use the same features as used in~\cite{Kalogeiton20,ball}. 
For the remaining datasets, we follow~\cite{Cao18} by expanding the face detection and taking a 224 x 224 centre crop for feature extraction. 
For \textit{Another Miss Oh!} (8), face-tracks are provided at 3FPS. 
We provide new face-tracks at 25FPS, by detecting faces using a RetinaFace architecture~\cite{deng2019retinaface}, with Mobilenet0.25~\cite{howard2017mobilenets} as the backbone network, trained on the WIDER FACE dataset~\cite{yang2016wider}. Face detections are linked into face-tracks, using a combination of IOU (intersection over union) and similarity between face embeddings to link detections. These are then automatically assigning each track to the 3FPS tracks provided by the dataset using temporal IOU.

\paragraph{Body-Tracks.}
Body-tracks are annotated using a three step process. 
First, bodies are detected in all frames using a Cascade R-CNN~\cite{cai2018cascade} trained with the body annotations in MovieNet~\cite{huang2020movienet}. 
Secondly, the detections are linked into body-tracks across frames. 
This is done with a simple IOU tracker, and by using the shot boundaries to prevent bodies from being tracked across shot changes. 
Thirdly, body tracks are annotated by assigning them to labelled face-tracks via a two stage process. The first stage is automatic. In each shot, the temporal IOU between each body-track and the annotated face-tracks is computed, and the Hungarian algorithm~\cite{kuhn1955hungarian} is used to make correspondences. In any case where multiple face-tracks intersect with the same body-track or vice versa, we do not make an assignment, this results in \~90\% of face-tracks being assigned body-tracks. The second stage is manually assigning the remaining body-tracks to face-tracks. Although \textit{Another Miss Oh!} provides body-tracks at 3FPS, we re-track and annotate the bodies using the detector that the body feature extractor was trained on.

\paragraph{Body-Features.}
Features are extracted from each of the body-tracks using a ResNet50 architecture. Our goal is to train the body features to discriminate identity based on the highly discriminative clothing that people are wearing. 
So, we train ResNet50 on a dataset where each class contains body detections of a person in movies wearing the same outfit. The dataset is made from the CSM dataset~\cite{huang2018person}, which contains body detections annotated with identity from movies. In CSM, the same person is annotated wearing many different outfits, so we decompose the samples for each class (identity) in CSM into sub-classes containing images of the same identity in the same outfit. We do this using the intuition that if two detections occur close-by temporally within the same movie, then the person is likely to be wearing the same clothing. Each body detection is annotated with the shot that the detection is found in. 
We cluster the body detections in each class according to their temporal location in the movie, allowing two detections to merge if they are two shots or less apart in the movie. This results in several sub-classes for each identity, where they are wearing the same clothing. We train ResNet50 using the Multi-Similarity loss from~\cite{wang2019multi}. The training procedure pulls embeddings of positive pairs together (the same identity wearing the same clothing) and pushes embeddings for negative pairs apart (different identities). More details can be found in the supplementary material \todo{(maybe put all of this there, also it is not fair to compare my features and theirs because mine was trained with stronger loss function. I should really train theirs with MS as well).}

\paragraph{Speech-Turns \& Features.}
For each of the speaking face-tracks in the datasets, we extract one single temporally aggregated speech descriptor. 
In detail, this consists of two stages: ASD (Active Speaker Detection) and speaker embedding extraction. For the ASD, we use an audio-visual synchronisation framework proposed in~\cite{Chung16a,8682524}. This classifies when/if each of the face-tracks in the constituent datasets are speaking, and outputs corresponding audio segments (if the face-track is not speaking, then there is no outputted audio segment). 
The network takes as input a mouth-centred face-track, and outputs a confidence score that the video is synchronised with the audio for each 5 frame window in the face-track. For a face-track depicting an active speaker, the confidence is high, allowing for ASD classification. Face-tracks with more than 0.5 seconds of consecutive speech, with a confidence above a strict threshold are classified as speaking, and the audio track is clipped to that speaking part. A L2-normalised 512D speaker embedding is then extracted from the speech segment using a thin-ResNet-34~\cite{Xie19a,He16}, as described in~\cite{chung2020in}, which was trained on the VoxCeleb2 dataset~\cite{Chung18a}.

\subsubsection{Multi-modal bridging Ablation}
\label{subsub:ablation_bridging}
Table~\ref{tab:person_results} includes an ablation of the multi-modal cluster bridging, \ie using either the face-body or the face-voice bridges. 
All \mnameMM results are obtained using Stage 1, for high-precision clustering with face, and Stage 3, for clustering backs using body. 
In most cases, 
the multi-modal bridging (iv-vi) improves upon no bridging (iii). 
This shows that the multiple modalities capture important information for clustering. 
For the three movies this boost is significant, for instance +28\% for CP and +10\% CR for Hidden Figures. 
This is because the duration of movies is longer than of tv shows and hence, the scenes, viewpoints and conditions of people are more diverse.  
Thus, the face alone cannot address this variety, but the multi-modal bridges can. 

Using both bridging strategies (vi) significantly outperforms using one of them (iv, v). 
For TBBT and Buffy, adding both bridges (vi) leads to minor performance improvements compared to using only one (iv, v), as they already perform well, \ie WCP of ~97\% for TBBT and ~86\% for Buffy. 
For Sherlock and Friends, the performance gain is best revealed by NMI, CP and CR, \ie +1-3\%, +1-2\%, +1-2\% vs one bridge (iv, v), respectively. 
Note, WCP improves only slightly by multi-modal bridges. This is expected as the bridging of two high-precision clusters will not greatly affect the overall cluster purity, however it leads to increased NMI as there is less identity intersection between the resulting clusters.
For the three movies, we observe that multi-modal bridging boosts most results. 
For About Last Night, the face-body bridge brings the highest improvement as it is able to distinguish characters in the often low-lighting settings of bars/restaurants where their face is not discriminative. 
For Hidden Figures, however, the face-body bridges lead to a small boost, as for a large part of the movie, many main characters wear the same outfit (\ie black and white costume)! In this case, the ratio-test ignores these non-distinctive body features. The face-voice bridge impacts the results much more, up to 28\% of CP.

\noindent \textbf{Face-less person-clustering.}
Table~\ref{tab:back_accuracy} reports classification accuracy results for the face-less body clustering. 
A face-less body is correctly classified if it is assigned to a body of the same identity. 
We classify them using the body features and the editing video structure, \ie if a frontal view of the same identity wearing the same clothes is found in a near-by shot. 
For the situational comedies (\eg Friends, Buffy), this is often the case (Figure~\ref{fig:backs}). 
The movies, however, are more challenging, as characters change clothing frequently and the changes between camera shot are less structured.
\todo{COMMENT ON NUMBERS}

\begin{figure}[t]
\begin{center}
\includegraphics[width=\linewidth]{figures/backsv1-2.pdf}
\end{center}
  \caption{\small{\textbf{First NN for backs}.  
  Exploiting the video editing structure allows for correct clustering of backs: (a) Ross, (b) Joey, and (c) Monica from \dnameemphasis.  }}
\label{fig:backs}
\end{figure} 

\begin{table}[]
\centering
\resizebox{\linewidth}{!}{
\begin{tabular}{l|rrrrrrrrrrrrrrr}
\toprule
dataset       & \cellcolor{lavenderblue}{TBBT} &  & \cellcolor{lavenderblue}{Buffy} & & \cellcolor{lavenderblue}{Sherlock} & & \cellcolor{lavenderblue}{Friends} & & \cellcolor{lavenderblue}{ALN} &  & \cellcolor{lavenderblue}{HF} & & \cellcolor{lavenderblue}{Hannah} & & \cellcolor{lavenderblue}{AVG} \\ \midrule
Accuracy &   xx  & &  xx   &  &  xx   &   &  xx  & &xx &  & xx & & xx &&   xx   \\
Ignored  &   xx  & &  xx   &  &  xx   &   &  xx  & &xx &  & xx & & xx && xx  \\ \bottomrule
\end{tabular}
}
\caption{\footnotesize{\textbf{Back-body clustering accuracy.} For each dataset in \dnameemphasis, the \% accuracy for clustering backs of bodies in Stage 3, along with the \% proportion of bodies not assigned a label for lack of confidence.}}
\label{tab:back_accuracy}
\end{table}

\ifx

\subsection{Face Clustering}
\label{sub:res_faceclustering}
%%%%%%%%%%%%%%%%%%%%%%%%%%%%%%
Table~\ref{tab:face_results} reports the results for face clustering. 
Recall that we evaluate two test protocols: (AT) automatic termination, unknown number of clusters, and (OC) oracle, known number of clusters. 
\mnameMM-- signifies the proposed method only by using information from the face-tracks. 
\mnameMM (bridges) signifies the additional use of the multi-modal bridges, both face-body and face-voice. For OC, \mnameMM-- and \mnameMM outperform the state of the art by a large margin. 
Note that \mnameMM-- has access to exactly the \emph{same} information as other methods, and therefore the results are directly comparable. 
For instance, for OC, there is an average of a 4\% boost in WCP across the four datasets, a 14\% boost in NMI for Buffy and TBBT, and over a 13\% improvement in CP and CR. 
This shows that the high-precision clustering averts incorrect merges, hence maintaining better purity clusters. 

\mnameMM (bridges) leads to further boosts for several datasets, \eg +2.5\% in CR for Friends and +3.7\% in NMI for Sherlock. 
Here, the extra modalities help distinguishing identities that the face alone cannot, thus underlying the benefits of multi-modal clustering.

For AT, both \mnameMM-- and \mnameMM (bridges)  consistently outperform the state of the art, \ie on average +19\% NMI and +7.5\% WCP across all datasets. 
By prioritising high-precision, they predict more clusters than characters, however only by a small margin. 
For instance, for TBBT, only 9-12 extra clusters are predicted (130 vs 139 and 142), and for Buffy only 32 (165 vs 197), whereas BCL predicts 92 too few clusters for TBBT and 94 for Buffy. 
%High purity is expected when predicting more clusters, but the fact that NMI increases significantly as well is an indication of the quality of the clustering, showing that there is far less class intersection between clusters for \mnameMM--. % --> moved to discussion 
For real-world scenarios, this is preferable, as a user chooses among slightly more high quality clusters, rather than fewer, far worse quality. 
The multiple modalities further move the predicted cluster number closer to the ground truth.

\noindent
\textbf{Discussion.}
Both C1C and BCL~\cite{ball} continue using face appearance even when the distances are large and features can no longer discriminate between clusters of the same identity, and therefore degenerate in the later partitions, leading to lower WCP (Figure~\ref{fig:cluster_example}). Instead, \mnameMM either terminates clustering once face appearance is no longer discriminatory, or furthermore leverages multi-modal information for better clustering. Part of the goal of BCL is to estimate the number of clusters. However, Table~\ref{tab:face_results} reveals that our estimation is superior.  
Furthermore, \mnameMM uses only pre-trained features, thus alleviating the computational burden, allowing for greater generalisation, and leading to better results with no learning. 
Note, the formulation of the NN distance constraint produces a similar constraint to that of BCL, which constrains fine-tuned features to a fixed-radius hyper-sphere.  
Importantly, we arrive at our formulation from a different direction, \ie  maintaining high precision and avoiding any incorrect merges that occur with large distances. In contrast to BCL and \mnameMM, C1C does not contain any hyper-parameters. Nevertheless, we argue that the vastly improved performance over the wide range of datasets justifies including them. Moreover, the ablation shows low performance sensitivity from their choice.

\fi 

\subsection{Metrics}
\label{sub:metrics}
%%%%%%%%%%%%%%%%%%
For each dataset in \dnameemphasis, we measure each metric at the episode level and then report the \% averaged over all episodes. 
Following~\cite{Kalogeiton20,ball}, we use Weighted Cluster Purity and Normalized Mutual Information. 
Furthermore, we introduce the metrics of Character Precision and Recall.%, as well as Fairness Score.  

\noindent \textbf{Weighted Clustering Purity (WCP).}
WCP weights the purity of a cluster by the number of samples belonging in it; to compute purity, each cluster $c$ containing $n_c$ elements is assigned to the class which is most frequent in the cluster. WCP is highest at 1 when within each cluster, all samples are from the same class. For a given clustering, $\mathcal{C}$, with $\mathcal{N}$ total tracks in the video: $WCP = \frac{1}{N} \sum_{c \in C}^{}  n_c \cdot purity_c $.

\noindent \textbf{Normalized Mutual Information (NMI)~\cite{manning2008introduction}.}
NMI measures the trade-off between clustering quality and number of resulting clusters. 
Given class labels $Y$ and cluster labels $C$, $\text{NMI}(Y,C) = 2\frac{I \left( Y ; C\right)}{ H(Y) + H(C)}$, where $H(.)$ is the entropy and $I(Y;C)=H(Y) - H(Y \backslash C)$ the mutual information.

\noindent \textbf{Character Precision and Recall (CP, CR).}
We introduce Character Precision (CP) and Recall (CR), two metrics computed using the ground truth number of clusters. 
CP is the proportion of tracks in a cluster that belong to its assigned character, 
while CR is the proportion of that character's total tracks that appear in the cluster. 
The assignment is done using the Hungarian algorithm~\cite{kuhn1955hungarian} by using CR as the cost function. 
Note that this assignment is unique, \ie two characters cannot be assigned to the same cluster. 
We measure CP and CR and report results averaged across all characters. 
Our intuition is that the standard metrics are weighted according the number of samples in each cluster, thus disproportionately favouring frequently appearing characters and disregarding tail distributions. 
Instead, similar to character AP~\cite{Nagrani17b}, CP and CR weight all characters equally. 
Similar to the Hungarian matching accuracy used in ~\cite{asano2020labelling,van2020learning}, CP and CR are computed using the ground truth number of clusters. 
Thus, they measure complementary information to WCP and NMI, which do not have access to this information.

\subsubsection{Ablation of parameters}
\label{subsub:ablation_params}
%\st{There are several hyper-parameters associated with the method. Here, we demonstrate the effects on some of the test datasets. We provide studies on the choice of the NN distance threshold $\tau_f^{\text{tight}}$, the ratio-test parameter $\rho$ and the modality bridge parameters. Further details can be found in the supplementary material.}
First, the nearest neighbour distance threshold,  $\tau_f^{\text{tight}}$. A high value allows for incorrect merging of clusters of different identities that are far apart. A value too low which leads to a strict stopping criterion that stops merging clusters too early. This is shown in Figure~\ref{fig:cluster_example} (right). The value is chosen as a balance between these two factors. Similarly for the multi-modality bridging thresholds, $\tau_f^{\text{loose}}$, $\tau_v^{\text{tight}}$,  $\tau_b^{\text{tight}}$, lower values indicate a stricter threshold on the distance between tracks. We find that for high values for $\tau_v^{\text{tight}}$ and $\tau_b^{\text{tight}}$, many false positive bridges are made and clustering quality decreases. This is because for the less discriminative modalities of body and voice, a low similarity cannot be taken as a confident indicator of two tracks being from the same identity. By keeping  $\tau_v^{\text{tight}}$ and $\tau_b^{\text{tight}}$ low (0.4 and 0.35, respectively) and raising the face threshold to $\tau_f^{\text{loose}} = 0.55$, the optimal balance is struck, where both modalities confidently agree to bridges between clusters that the face modality alone could not bridge. Full quantitative analysis can be found in the supplementary material.

\begin{figure}[t!]
\begin{center}
\includegraphics[width=\linewidth]{figures/ablation.pdf}
\end{center}
\vspace{-7mm}
  \caption{\footnotesize{\textbf{\%WCP for Buffy ep.\ 2} (left) Comparisons to previous methods w/,w/o automated termination (right) varying values of $\tau_f^{\text{tight}}$.}}
\label{fig:cluster_example}
\end{figure}

\paragraph{body assignment}
The body-tracks of all annotated characters fall into two categories, which are annotated separately.
(1) The body-track shows the person from the front and contains a visible, annotated face. For these cases we automatically label body-tracks by making assignments to labelled face-tracks. Within each shot, the assignment is done using the Hungarian Algorithm~\cite{kuhn1955hungarian} with a cost function of the spatial intersection over union (IOU) between face and body tracks in the frames that they co-occur. If there are more body-tracks than face-tracks, then a body-track can not be assigned, and vice-versa. In ~95\% of cases this association is trivial and the assignment proceeds automatically. Where multiple assignment costs for the same face-track are below a threshold, indicating that the assignment was non-trivial, we make the assignments manually. 
(2) The body-track does not contain a visible face, \ie the back is turned to the camera. We manually annotate all of these cases throughout each video. Due to common TV-show/movie editing structures, these cases are less likely, and are usually found when a character walks off scene, or from an \textit{over-the-shoulder} camera-shot. On average, 10-15\% of body-tracks correspond to manually labelled bodies from behind.

% Interestingly, for Friends and Sherlock, using both types of bridges where the combination of the two bridging methods results in a higher score than using one alone. This shows that the face-body bridges and the face-voice bridges are linking different clusters, and one is not a subset of the other. 

\ifx
\subsection{Discussion}
\label{sub:res_dicussion}
%%%%%%%%%%%%%%%%%%%%%%%%%%%%%%
\mnameMM shows significant boosts over all baselines, ablations and previous methods for both face-clustering and person-clustering. 
Furthermore, using extra modalities leads to a consistent advantage. 
The person-clustering results (Table~\ref{tab:person_results}) show that there is room for improvement. 
%Particularly from extending the lengths of the videos being clustered by concatenating different TV-shows and movies and viewing the effect on the clustering performance. 

\noindent \textbf{Metric assessment.}
Interestingly, for both AT and OC protocols, the WCP results are much higher than other metrics (\eg +8-17\% in Table~\ref{tab:person_results}). 
This shows that WCP \emph{alone} is not suitable for measuring the clustering performance, even when evaluating on the oracle number of clusters (OC), thus highlighting the importance of our additional CP and CR metrics. 
For AT, when predicting more clusters (est \#C is higher than the oracle \#C) high purity is expected. 
Notably, in all cases NMI also increases, thus indicating the high clustering quality, showing that there is far less class intersection between clusters for our method.
%Moreover, high purity is expected when predicting more clusters, but the fact that NMI increases significantly is an indication of the quality of the clustering, showing that there is far less class intersection between clusters for \mnameMM--. 
 \fi
